# Supplementary material for: Disadvantaged students increase their academic performance through collective intelligence exposure in emergency remote learning due to COVID 19
Source: arXiv:2203.05621 source file (2022-03-10)
Supplement: Supplementary file 1 [file main_fig_SM.pdf]

# Hierarchical Regression Coefficients (fixed effects)

A

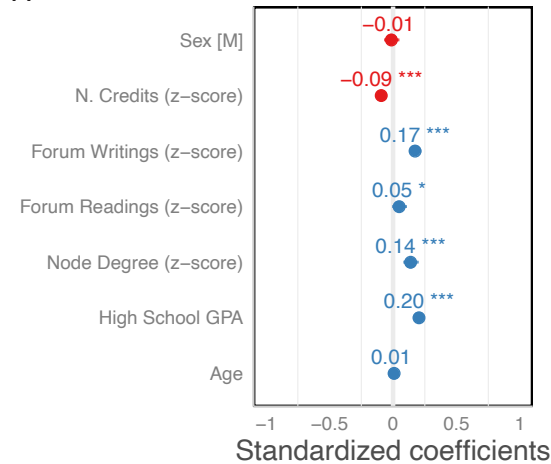

B

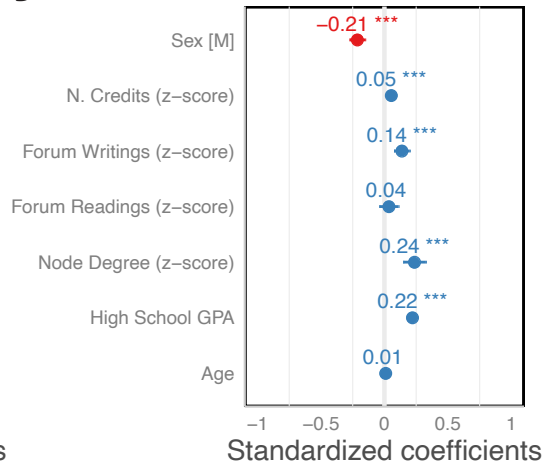

C

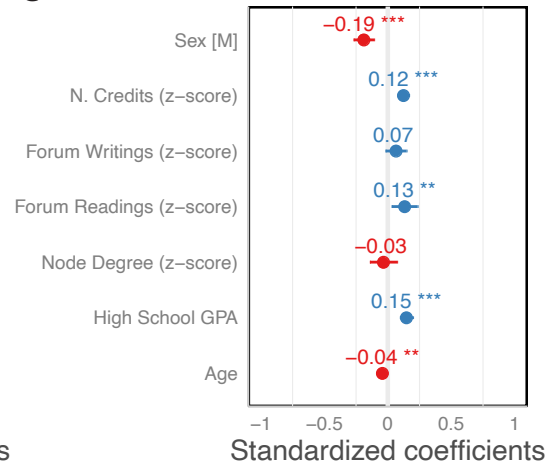

## Marginal Effects

D

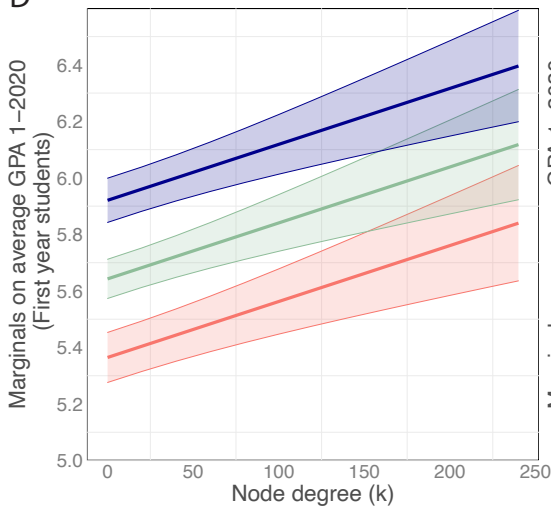

E

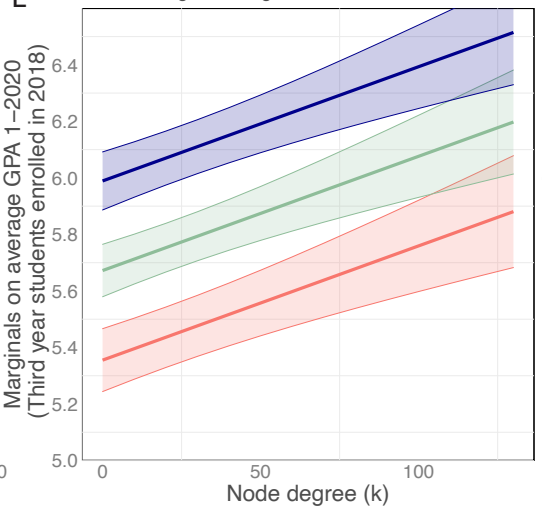

F

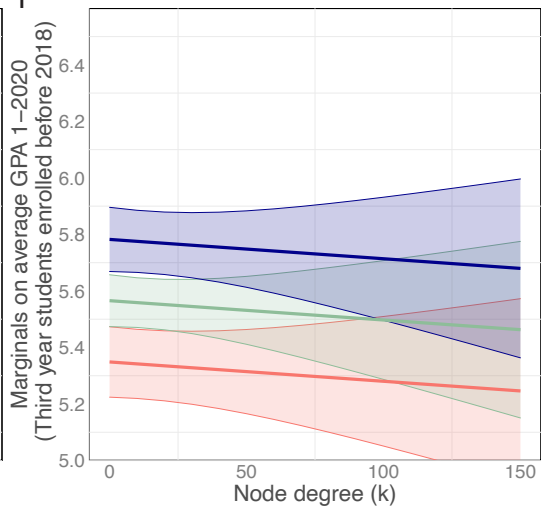

# Marginal Effects
